# Supplementary material for: Data Poisoning Attacks to Local Differential Privacy Protocols for Graphs
Source: arXiv:2412.19837 source file (2024-12-23)
Supplement: Supplementary file 1 [file Appendix.tex]

\subsection{Proof of Theorem 1.}

\noindent
The overall gain of MGA to degree centrality is 
\begin{equation}
\text{Gain} = \frac{m \cdot r}{N-1} \cdot \bigg(\frac{\min(r, \lfloor\overline{\tilde{d}}\rfloor)}{r} - \frac{\overline{\tilde{d}}}{N-1}\bigg)  \nonumber
\end{equation}
where $\overline{\tilde{d}}$ is the average degree of the graph after perturbation.
\begin{proof}
To prove this theorem, we begin by considering the probability of an existing connection between any two nodes, which is $p' = \frac{\overline{\tilde{d}}}{N-1}$. Next, we consider the maximum number of new connections that can be added per fake node. Each fake node can add at most $\min(r, \lfloor\overline{\tilde{d}}\rfloor)$ connections, but we need to subtract the existing connections. Thus, the maximum number of new connections per fake node is $\min(r, \lfloor\tilde{d}\rfloor) - p \cdot r$.

Extending this to all fake nodes, the total number of new connections that can be added is
$E_{\text{new}} = m \cdot \left(\min(r, \lfloor\overline{\tilde{d}}\rfloor) - p \cdot r\right) = m \cdot \left(\min(r, \lfloor\overline{\tilde{d}}\rfloor) - \frac{r\overline{\tilde{d}}}{N-1}\right)$.

We now consider the impact on degree centrality. When a single node's degree increases by $1$, its degree centrality changes by $\frac{1}{N-1}$. Therefore, the overall gain in degree centrality for all target nodes can be expressed as $\text{Gain} = \frac{E_{\text{new}}}{N-1}$. Substituting the expression for $E_{\text{new}}$, we have
$\textit{Gain} = \frac{m}{N-1} \cdot (\min(r, \lfloor\overline{\tilde{d}}\rfloor) - \frac{r\overline{\tilde{d}}}{N-1}) = \frac{m \cdot r}{N-1} \cdot (\frac{\min(r, \lfloor\overline{\tilde{d}}\rfloor)}{r} - \frac{\overline{\tilde{d}}}{N-1})$.
\end{proof}

\subsection{Proof of Theorem 2.}

\noindent

\begin{figure}
    \centering
    \begin{subfigure}[b]{0.98\linewidth}
        \centering
    \includegraphics[width=\linewidth]{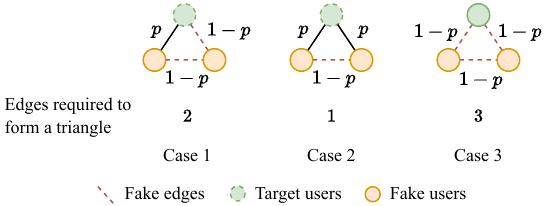}
    \end{subfigure}
    \caption{Edges required to form a triangle.}
    \label{fig:triangle-three-cases}
\end{figure}

\noindent
The overall gain of MGA to the clustering coefficient is 
\begin{align*}
\text{Gain} &= r \cdot \frac{2}{p^2(2p - 1)} \cdot \frac{1}{\overline{\widetilde{d}}(\overline{\widetilde{d}}-1)} \\
&\cdot \frac{m}{2 \cdot p'(1-p')^2 + p'^2(1-p')+3\cdot(1-p')^3} \nonumber
\end{align*}
where $\overline{\tilde{d}}$ is the average perturbed degree and $p' = \frac{\overline{\tilde{d}}}{N-1}$ is the probability of forming a connection.
\begin{proof}
We begin by considering the probability of a connection, given by $p' = \frac{\overline{\tilde{d}}}{N-1}$, where $\overline{\tilde{d}}$ is the average perturbed degree and $N$ is the total number of nodes. To estimate the probability of forming a triangle, we should consider three possible scenarios, as shown in Fig. \ref{fig:triangle-three-cases}. Observe that the probability is $p'^2(1-p')$ when two edges already exist (Case 2). Similarly, the probability is $2 \cdot p'(1-p')^2$  when one edge exists (Case 1) and $3 \cdot (1-p')^3$ when no edges exist (Case 3), respectively. Given $m$ fake nodes, each target node can have $m$ connections with fake nodes. Consequently, the number of new triangles to be introduced is $\frac{m}{2 \cdot p'(1-p')^2 + p'^2(1-p') + 3 \cdot (1-p')^3}$.

For a target node $i$, the difference of clustering coefficient $cc_i$ before and after the attack can be expressed as $\frac{2}{p^2(2p - 1)} \cdot \frac{1}{\widetilde{d_i}(\widetilde{d_i}-1)} \cdot \frac{m}{2 \cdot p'(1-p')^2 + p'^2(1-p') + 3 \cdot (1-p')^3}$, where $\widetilde{d_i}$ represents the perturbed degree for node $i$. Since there are $r$ target nodes, the overall gain is therefore $r \cdot \frac{2}{p^2(2p - 1)} \cdot \frac{1}{\widetilde{d}(\widetilde{d}-1)} \cdot \frac{m}{2 \cdot p'(1-p')^2 + p'^2(1-p') + 3 \cdot (1-p')^3}$.
\end{proof}
